# Supplementary material for: GPT Understands, Too
Source: arXiv:2103.10385 source file (2023-10-25)
Supplement: Supplementary file 1 [file 7_appendix.tex]

\section{Appendix}

\subsection{Hyper-parameters for Few-Shot Learning}\label{sec:fewshothparam}

We list the hyper-parameter space for few-shot learning experiments in Table~\ref{tab:fewshotsearchspace}.
\begin{table}[htbp]
\small
\centering
\resizebox{\linewidth}{!}{%
  \begin{tabular}{l|ccccccc}
    \toprule[1pt]
    Hyper-parameter & Value \\ 
    \midrule
    Learning Rate & $\{1e-5, 2e-5\}$\\
    Maximum Training Step &  $\{250, 500\}$\\
    Evaluation Frequency & $\{0.02, 0.04\}$\\
    Number of Runs $K$ & 4 \\
    Split Ratio $r$ & 1:1 \\
    % Patterns & As~\cite{schick2020small} \\
    Prompt Type (\solution) & \{LSTM, MLP, EMB\} \\
    Number of Cont. Tok. (\solution) & \{1\} \\
    \bottomrule[1pt]
\end{tabular}
}
\caption{Hyper-parameter search space for few-shot experiments. The patterns are same as ~\cite{schick2020small}.}
\label{tab:fewshotsearchspace}
\end{table}
